# Supplementary material for: Contrastive Deep Learning Reveals Age Biomarkers in Histopathological Skin Biopsies
Source: arXiv:2411.16956 source file (2026-07-01)
Supplement: Supplementary file 1 [file appendix.tex]

%To include, in this order: \textbf{Accession codes} (where applicable); \textbf{Competing interests} (mandatory statement). 

%The corresponding author is responsible for submitting a \href{http://www.nature.com/srep/policies/index.html#competing}{competing interests statement} on behalf of all authors of the paper. This statement must be included in the submitted article file.
