# Supplementary material for: Contrastive Deep Learning Reveals Age Biomarkers in Histopathological Skin Biopsies
Source: arXiv:2411.16956 source file (2026-07-01)
Supplement: Supplementary file 2 [file supplementary.tex]

\documentclass[12pt]{article}

\usepackage{graphicx}
\usepackage{booktabs}
\usepackage{float}
\usepackage{amsmath}
\usepackage{hyperref}
\usepackage{geometry}

\geometry{margin=1in}

\begin{document}

\title{Supplementary Material for the manuscript Histological Ageing Signatures in Routine Skin Biopsies Are Associated with Disease Burden and Mortality}
\maketitle

\input{10_supplementary}

\end{document}
